# Supplementary material for: RADIUS: Risk-Aware, Real-Time, Reachability-Based Motion Planning
Source: arXiv:2302.07933 source file (2023-06-19)
Supplement: Supplementary file 1 [file appendix_control.tex]

\section{Trajectory Parametrization and Control}
\label{app: control}

This work adapts trajectory parametrization and control from \cite{REFINE}.
We start by formally define a desired trajectory as follows:
\begin{defn}\label{def:traj_param}
For each $p \in \P$, a \emph{desired trajectory} is a function for the longitudinal speed, $\udes(\cdot,p):[\tz+\tplan,\tz+\tplan+t_\text{f}] \to \R$, a function for the heading, $\hdes(\cdot,p):[\tz+\tplan,\tz+\tplan+t_\text{f}] \to \R$, and a function for the yaw rate, $\rdes(\cdot,p): [\tz+\tplan,\tz+\tplan+t_\text{f}] \to \R$, that satisfy the following properties.
\begin{enumerate}
% We require that $q_d(\cdot; k): T \to Q$ satisfies three properties for all $k \in K$
\item For all $p\in\P$, there exists a time instant $\tnb\in[\tz+\tplan,\tz+\tplan+\tf)$ after which the desired trajectory begins to brake (i.e., $|\udes(t,p)|$, $|\hdes(t,p)|$ and $|\rdes(t,p)|$ are non-increasing for all $t\in[\tnb,\tz+\tplan+\tf]$).
\item The desired trajectory eventually comes to and remains stopped (i.e., there exists a $\tstop \in [\tz+\tplan,\tz+\tplan+\tf]$ such that $\udes(t, p) = \hdes(t, p) = \rdes(t, p) = 0$ for all $t \geq \tstop$).
\item $\udes$ and $\hdes$ are piecewise continuously differentiable \cite[Chapter 6, $\S$1.1]{remmert1991theory} with respect to $t$ and $p$.
\item The time derivative of the heading function is equal to the yaw rate function (i.e., $\rdes(t,p)=\frac{\partial}{\partial t}\hdes(t,p)$ over all regions that $\hdes(t,p)$ is continuously differentiable with respect to $t$).
% \item $q_d(\cdot; k) $ is at least once-differential with respect to time (i.e., no discontinuities in joint position or velocity).
% \pat{Third, $q(0; k) = 0$ (each joint starts from zero initial angle).}
\end{enumerate}
\end{defn}
\noindent The first two properties ensure that a fail safe maneuver is always available due to the safety concern of not-at-fault, and the latter two properties ensure that the tracking controller described next is well-defined.
Note that sometimes we abuse notation and evaluate a desired trajectory for $t > \tf$.
In this instance, the value of the desired trajectory equals to its value at $\tf$.

Next we describe the tracking controller, and we start by introducing the controller on longitudinal speed whose dynamics appears in both high-speed and low-speed models.
We set the longitudinal front tire force to be:
\begin{equation}
    \label{eq: Fxf}
    \begin{split}
    F_\text{xf}(t) = -m K_u (u(t) - \udes(t,p) ) + m\dudes(t,p) + \\ - F_\text{xr}(t)- mv(t)r(t) + m\tau_u(t,p),
    \end{split}
\end{equation}
where
\begin{align}
\tau_u(t,p) =& -\big(\kappa_u(t,p) M_u+\phi_u(t,p)\big)e_u(t,p), \label{eq: tau_u def} \\
    \kappa_u(t,p) =& \kappa_{1,u}+\kappa_{2,u}\int_{\tz}^t\|u(s)-\udes(s,p)\|^2ds,\label{eq: kappa_u def}\\
    \phi_u(t,p) =&\phi_{1,u}+\phi_{2,u}\int_{\tz}^t\|u(s)-\udes(s,p)\|^2ds,\label{eq: phi_u def}\\
    e_u(t,p) =& u(t)-\udes(t,p), \label{eq: e_u def}
\end{align}
with user-chosen constants $K_u,\kappa_{1,u},\kappa_{2,u},\phi_{1,u},\phi_{2,u}\in\R_+$ where $\R_+$ indicates the space of non-negative real numbers.
Note in \eqref{eq: Fxf} we have suppressed the dependence on $p$ in $F_\text{xf}(t)$ for notational convenience.
Using \eqref{eq: Fxf}, the closed-loop dynamics of $u$ become: 
\begin{equation}
\begin{split}
    \dot u(t) = \tau_u(t,p) + \Delta_u(t) + \dudes(t,p) + \\ -K_u \left( u(t) - \udes(t,p)\right).
    \end{split}
    \label{eq: u_dot_closed_loop_eq}
\end{equation}

The same control strategy can be applied to vehicle yaw rate whose dynamics only appear in  the high-speed vehicle model.
Let the lateral front tire force be 
\begin{equation}
\label{eq: Fyf}
\begin{split}
    % F_\text{yf}(t) = \frac{1}{l_\text{f}}\big(I_\text{zz}\drexp(t,p)+ l_\text{r}F_\text{yr}(t) + I_\text{zz}\varphi_r(t,p) \big)
     F_\text{yf}(t) = -\frac{I_\text{zz} K_r}{l_\text{f}}\left( r(t) - \rdes(t,p) \right) +  \frac{I_\text{zz}}{l_\text{f}} \drdes(t,p) + \\ -\frac{I_\text{zz} K_h}{l_\text{f}}\left( h(t) - \hdes(t,p)\right) + \frac{l_\text{r}}{l_\text{f}} F_\text{yr}(t) + \frac{I_\text{zz}}{l_\text{f}} \tau_r(t,p),
     \end{split}
    % \frac{I_\text{zz}}{l_\text{f}}\drexp(t;d) +\frac{l_\text{r}}{l_\text{f}} F_\text{yr}(t) + \frac{I_\text{zz}}{l_\text{f}}\varphi_r(t;d)
\end{equation}
where
\begin{align}
 \tau_r(t,p) =& -\big(\kappa_r(t,p) M_r+\phi_r(t,p)\big)e_r(t,p) \label{eq: tau_r def} \\
    \kappa_r(t,p) =& \kappa_{1,r}+\kappa_{2,r}\int_{\tz}^t\left\| \begin{bmatrix}r(s)\\h(s)\end{bmatrix} - \begin{bmatrix}\rdes(s,p)\\\hdes(s,p)\end{bmatrix}\right\|^2ds\\
    \phi_r(t,p) =&\phi_{1,r}+\phi_{2,r}\int_{\tz}^t\left\| \begin{bmatrix}r(s)\\h(s)\end{bmatrix} - \begin{bmatrix}\rdes(s,p)\\\hdes(s,p)\end{bmatrix}\right\|^2ds\\
    % e_r(t,p) =& K_r(r(t)-\rdes(t,p))+K_h(h(t)-\hdes(t,p)),
    e_r(t,p) =& \begin{bmatrix} K_r & K_h \end{bmatrix} \begin{bmatrix} r(t)-\rdes(t,p) \\ h(t)-\hdes(t,p) \end{bmatrix}
\end{align}
with user-chosen constants $K_h,K_r,\kappa_{1,r},\kappa_{2,r},\phi_{1,r},\phi_{2,r}\in\R_+$.
Note in \eqref{eq: Fyf} we have again suppressed the dependence on $p$ in $F_\text{yf}(t)$ for notational convenience.
Using \eqref{eq: Fyf}, the closed-loop dynamics of $r$ become:
\begin{equation}
    \begin{split}
    \dot r(t) = &\tau_r(t,p)+ \Delta_r(t)+ \drdes(t,p) + \\ & -K_r\big(r(t) - \rdes(t,p)\big)+  \\  &-K_h\big(h(t) - \hdes(t,p)\big).
    \end{split}
    \label{eq: r_dot_closed_loop_eq}
\end{equation}
Using \eqref{eq: Fyf}, the closed-loop dynamics of $v$ become:
\begin{equation}
    \begin{split}
        \dot v(t) = \frac{1}{m}\Bigg(\frac{l}{l_\text{f}} F_\text{yr}(t) +\frac{I_\text{zz}}{l_\text{f}}\Big(\tau_r(t,p) + \drdes(t,p) + \\
        - u(t)r(t)+\Delta_v(t) -K_r\big(r(t) - \rdes(t,p)\big) + \\ -K_h\big(h(t) - \hdes(t,p)\big) \Big) \Bigg).
    \end{split}
    \label{eq: v_dot_closed_loop_eq}
\end{equation}
