# Supplementary material for: RADIUS: Risk-Aware, Real-Time, Reachability-Based Motion Planning
Source: arXiv:2302.07933 source file (2023-06-19)
Supplement: Supplementary file 2 [file appendix_footprint.tex]

\section{Proof of Theorem \ref{thm:footprint}}
\label{app: proof of thm footprint}
\new{Before proving Theorem \ref{thm:footprint}, we first prove a lemma:}

\begin{lem}
    \label{lem: trajectories of different initial pos}
    \new{Given arbitrary $[x_0,y_0,h_0]^\top\in\R^3$, $\zvel_0\in\R^3$ and $p\in\P$, let $z$ and $\bz$ be solutions to \eqref{eq: vehicle dynamics} with initial conditions $z(0) = [x_0,y_0,h_0,(\zvel_0)^\top]^\top$ and $\bz(0) = [0,0,0,(\zvel_0)^\top]^\top$ respectively, then
     \begin{equation}
        \pi_{xy}(z(t)) = \rot(h_0)\cdot\pi_{xy}(\bz(t)) + [x_0,y_0]^\top.
    \end{equation}
    }
\end{lem}
\begin{proof}
    \new{Notice that $z(0)$ and $\bz(0)$ shares the same initial velocities, and that the dynamics of $[u,v,r]^\top$ is invariant to the initial condition of $[x,y,h]^\top$.
    Therefore the last 3 dimensions of $z(t)$ and $\bz(t)$ coincides for all $t$.
    Because $\dot h(t) = r(t)$, then 
    \begin{equation}
        [z(t)]_3 = [\bz(t)]_3 + h_0.
    \end{equation}
    Then the claim follows from the fact that 
    \begin{equation}
        \begin{bmatrix}
            \dot x(t)\\ \dot y(t)
        \end{bmatrix} = \begin{bmatrix}
            \cos(h(t)) & -\sin(h(t)) \\ \sin(h(t)) & \cos(h(t))
        \end{bmatrix} \begin{bmatrix}
            u(t) \\ v(t)
        \end{bmatrix}.
    \end{equation}
    }
\end{proof}

% \begin{rem}
%     \label{rem: trajectories of different initial pos}
%     Given arbitrary $x_0,y_0,h_0\in\R$ and $\zvel_0\in\R^3$, let $z$ and $\bz$ be solutions to \eqref{eq: dyn tilde_z} with control parameter $p$ and initial conditions $[x_0,y_0,h_0,(\zvel_0)^\top]^\top$ and $[0,0,0,(\zvel_0)^\top]^\top$, respectively.
%     Then based on the fact that dynamics of $[u,v,r]^\top$ are independent of $[x,y,h]^\top$ \Ram{I am not sure what independent means in this context} \challen{confusion stems from the fact that we are using Probabilities in this paper. Instead we should say is not dependent}\cite[(4)]{REFINE}, one can show that 
%     \begin{equation}
%         \pi_{xy}(z(t)) = \rot(h_0)\cdot\pi_{xy}(\bz(t)) + [x_0,y_0]^\top
%     \end{equation}
%     where $\pi_{xy}: \R^{6}\rightarrow \R^2$ \Ram{probably should define $\pi$ in the notation section} is the projection operator that outputs the first two coordinates from its argument.
% \end{rem}
% \Ram{you provide no context for this remark...}\jinsun{upgrade it to a lemma}
\new{Now we prove Theorem \ref{thm:footprint}.}
\begin{proof}
    For any $z(0) = z_0 = [x_0,y_0,h_0,(\zvel_0)^\top]^\top\in\R^3\times\Zvel_0$, let $\bz$ be the solution to \eqref{eq: vehicle dynamics} with initial condition $\bz(0) = [0,0,0,(\zvel_0)^\top]^\top$ with control parameter $p$.
    Then there exists a zonotope $\bxi(\RR_j,\zvel_0,p)\subset\W$ such that for any $j\in\J$ and $t\in T_j$, the vehicle footprint oriented and centered according to $\bz(t)$ is contained within $\bxi(\RR_j,\zvel_0,p)$ \cite[Lem. 21]{REFINE}.
    Let
    \begin{equation}
    \label{eq: xi def}
        \xi(\RR_j,z_0,p) := \rot(h_0)\cdot\bxi(\RR_j,\zvel_0,p) + [x_0,y_0]^\top,
    \end{equation}
    then $\xi(\RR_j,z_0,p)$ contains the vehicle footprint according to $\zaug(t)$ during $T_j$ based on Lemma \ref{lem: trajectories of different initial pos}.
    
    In addition, $\bxi(\RR_j,\zvel_0,p)$ is a zonotope and can be represented as $\zonocg{c_{\bxi,j}(\zvel_0)+ A_{\bxi,j}\cdot p}{G_{\bxi,j}}$ with some $c_{\bxi,j}(\zvel_0)\in\W$, some $A_{\bxi,j}\in\R^{2\times n_p}$ and some 2-row real matrix $G_{\bxi,j}$ \cite[Lem. 26]{REFINE}.
    Thus $\xi(\RR_j,z_0,p)$ is a zonotope of the form $\zonocg{c_{\xi,j}(z_0)+A_{\xi,j}\cdot p}{G_{\xi,j}}$ where
    \begin{equation}
        \begin{cases}
            c_{\xi,j}(z_0) = \rot(h_0)\cdot c_{\bxi,j}(\zvel_0) + [x_0,y_0]^\top\\
            A_{\xi,j} = \rot(h_0)\cdot A_{\bxi,j}\\
            G_{\xi,j} = \rot(h_0)\cdot G_{\bxi,j}
        \end{cases}.    
    \end{equation}
\end{proof}
