# Supplementary material for: RADIUS: Risk-Aware, Real-Time, Reachability-Based Motion Planning
Source: arXiv:2302.07933 source file (2023-06-19)
Supplement: Supplementary file 3 [file appendix_thresholdproof.tex]

\section{Proof of Theorem \ref{thm:threshpandz0}}
\label{app: proof of thm threshpandz0}
% \begin{thm} %THM 14
% There exists some piece-wise differentiable function $\epszp$ such that $\epszp=\inf_{t\in[0,\tm]}\big(\dyneps(u(t))\big)$
% \end{thm}

To prove Theorem \ref{thm:threshpandz0} we must first introduce the following two assumptions:

\begin{assum}
\label{ass: udeszp}
    From \cite[Eqn. 57]{REFINE} we have that $u^{des}(t)$ is a linear operator of $z_{0}$ and p, $\forall t\in[0, \tf]$
\end{assum}

\begin{assum}
\label{ass: ubound}
    Additionally, from \cite[Appendix A]{REFINE} the tracking error $|u^{des}(t) - u(t)|$
    of the robust controller is bounded above by some threshold $u_{small},$ such that  $|u^{des}(t) - u(t)| \leq u_{small}$ $\forall t \in [0, \tm]$
\end{assum}

\begin{proof}

From Assumption \ref{ass: udeszp}, the desired trajectory longitudinal velocity is a linear operator of $z_{0}$ and p, $\forall t\in[0, \tf]$.
Based on the reasoning of Assumption \ref{ass: ubound}, the tracking error $|u^{des}(t,p) - u(t)|$ of the robust controller is bounded above by $u_{small}$, i.e. $u^{des}(z_0,p) - u_{small} \leq u(t) \leq u^{des}(z_0,p) + u_{small}$, for all $t\in[0,\tm]$.

Because we have a closed form representation of $\dyneps$ as in \eqref{eq: def dyneps}, we know its monoticity at every point. 
For $u(t)\in [0, 31.5)$ [mph] it is monotonically increasing, for $u(t)\in (31.5, 59.6)$ [mph] it is monotonically decreasing, and for $u(t) \in (59.6, 67.1]$ [mph] it is monotonically increasing.

Let $a(z_0,p) = \dyneps\big(\min_{t\in[0,\tm]} u^{des}(t,z_0,p)-u_{small}\big) $ and let $b(z_0,p) = \dyneps\big(\max_{t\in[0,\tm]} u^{des}(t,z_0,p) + u_{small}\big).$
Let $\underline{u} = \min_{t\in[0,\tm]} u(t)$ and let $\overline{u} = \max_{t\in[0,\tm]} u(t).$
Assuming our vehicle can only reach a maximum velocity of 67.1 [mph], then $\epszp = \inf_{t\in[0,\tm]}\big(\dyneps(u(t))\big)$ is given as:
\begin{equation}
\label{eq: eps value}
     \epszp =  \begin{dcases}
        a(z_0,p), \text{ if } a(z_0,p) \leq b(z_0,p)~and~59.6 \notin [\underline{u}, \overline{u}]\\
        b(z_0,p), \text{ if } a(z_0,p) > b(z_0,p)~and~59.6 \notin [\underline{u}, \overline{u}]\\
        \dyneps(59.6) ~ \text{ otherwise }
    \end{dcases}.
\end{equation}

Notice that $\dyneps$ is a polynomial and thus differentiable. 
We denote $\frac{\partial\dyneps}{\partial u}( \min_{t\in[0,\tm]} u^{des}(t,z_0,p)-u_{small})$ as $\frac{\partial\dyneps_{min}}{\partial u}(z_0,p)$ and denote $\frac{\partial\dyneps}{\partial u}( \max_{t\in[0,\tm]} u^{des}(t,z_0,p)+u_{small})$ as $\frac{\partial\dyneps_{max}}{\partial u}(z_0,p)$.
We further simplify notation in the remainder of this section by denoting $\frac{\partial\dyneps_{min}}{\partial u}(z_0,p)$ as $\frac{\partial\dyneps_{min}}{\partial u}$ and denoting $\frac{\partial\dyneps_{max}}{\partial u}(z_0,p)$ as $\frac{\partial\dyneps_{max}}{\partial u}$.

% $\frac{\partial\dyneps}{\partial u}( \min_{t\in[0,\tm]} u^{des}(t,z_0,p)-u_{small})$ as $\frac{\partial\dyneps_{min}}{\partial u}(z_0,p)$ and denote $\frac{\partial\dyneps}{\partial u}( \max_{t\in[0,\tm]} u^{des}(t,z_0,p)+u_{small})$ as $\frac{\partial\dyneps_{max}}{\partial u}(z_0,p)$.
Then
\begin{equation}
\label{eq: deps value}
     \frac{\partial \epsilon}{\partial p}(z_0,p) =  \begin{dcases}
        \begin{split}
            &\frac{\partial\dyneps_{min}}{\partial u} \cdot \frac{\partial \udes}{\partial p}(t,z_0,p), \text{ if } a(z_0,p) \leq b(z_0,p)\\
            &\hspace{4cm}~and ~59.6 \notin [\underline{u}, \overline{u}]\\
            &\frac{\partial\dyneps_{max}}{\partial u}\cdot \frac{\partial \udes}{\partial p}(t,z_0,p), \text{ if } a(z_0,p) > b(z_0,p)\\
            &\hspace{4cm}and~59.6 \notin [\underline{u}, \overline{u}]\\
            &0, \text{ otherwise } \\  
        \end{split}
    \end{dcases}.
\end{equation}

\end{proof}
