# Supplementary material for: RADIUS: Risk-Aware, Real-Time, Reachability-Based Motion Planning
Source: arXiv:2302.07933 source file (2023-06-19)
Supplement: Supplementary file 5 [file appendix_conservativeness.tex]

\section{Conservatism on Risk Evaluation}
\label{app: conservatism}
Although previous experimental results have shown that \riskmethodname{} outperforms mentioned stochastic and deterministic approaches, the resulting crash rate utilizing \riskmethodname{} is considerably small compared against the value of allowable risk threshold ($\epsilon$) we specified in experiments. 
This suggests that our risk approximation is

\begin{rem}
    To achieve a tighter upper bound of $\pdf$ on $\T+A_{j}p$, one can replace $H_\T$ in \eqref{eq: f after IA} by some matrix $\tilde H_\T(p)\in\R^{2\times 2}$, which is computed by taking element-wise supremum of the Hessian of $\pdf$ over $\T+A_{j}p$ instead of $\T\oplus A_{j}\PP$ using interval arithmetic.
    However, recall that we aim to over approximate $\int_{\xi_j(z_0,p)\oplus\zonocg{0}{\Gobs}} \pdf(w) ~dw$ with a closed form representation while preserving differentiability.
    Unfortunately taking the derivative of $\tilde H_\T(p)$ with respect to $p$ is challenging when using interval arithmetic.
    On the other hand, the derivative of $H_\T$ with respect to $p$ is $0$ because by construction $H_\T$ is invariant over $\PP$.
    % \new{Hence using $H_\T$ instead of $\tilde H_\T(p)$ is preferred.}
\end{rem}
