# Supplementary material for: RADIUS: Risk-Aware, Real-Time, Reachability-Based Motion Planning
Source: arXiv:2302.07933 source file (2023-06-19)
Supplement: Supplementary file 6 [file appendix_notatfault.tex]

\section{Proof of Theorem \ref{thm: risk condition}}
\label{app: proof of thm risk cond}

Before proving Theorem \ref{thm: risk condition}, we first present a pair of lemmas.
\begin{lem}
\label{lem: bring cup_i out}
    Suppose the ego vehicle starts with initial condition $z_0\in\Z_0$ and control parameter $p\in\PP$.
    % Let the collections of PDFs $\{\pdf\}_{(i.j)\in\I\times\J}$ and maps $\{\xi_j\}_{j\in\J}$ be as assumed in Assumptions \ref{ass: obs pdf} and \ref{ass: offline reachability}  respectively, and let matrix $\Gobs$ be as assumed in Assumption \ref{ass: swept_volume assumption}.
    Then for any $j\in\J$, 
    \begin{equation}
        \begin{split}
            \{t\in\ T_j \mid  \E(t,&z_0,p)\cap\big(\cup_{i\in\I}\Oobs(t) \big)  \} = \\
            &= \cup_{i\in\I}\{t\in T_j\mid \E(t,z_0,p)\cap\Oobs(t) \}.
        \end{split}
    \end{equation}
\end{lem}
\begin{proof}
    For notational simplicity let $\A_1:=\{t\in\ T_j \mid  \E(t,z_0,p)\cap\big(\cup_{i\in\I}\Oobs(t) \big)  \}$ and $\A_2:=\cup_{i\in\I}\{t\in T_j\mid \E(t,z_0,p)\cap\Oobs(t) \}$.  
    We prove the claim by showing $\A_1\subseteq\A_2$ and $\A_2\subseteq\A_1$
    
    For any $t' \in \A_1$, we have $\E(t',z_0,p)\cap\big(\cup_{i\in\I}\Oobs(t') \big) $, then there exists some $i'\in\I$ such that $\E(t',z_0,p)\cap \OO^\text{obs}_{i'}(t')$.
    In other words, 
    \begin{equation}
        t'\in\{ t\in T_j\mid \E(t,z_0,p)\cap \OO^\text{obs}_{i'}(t)\}\subset\A_2,
    \end{equation}
    therefore $\A_1\subseteq\A_2$.
    
    For any $t''\in\A_2$, by definition of $\A_2$ there exists some $i''\in\I$ such that $\E(t'',z_0,p)\cap \OO^\text{obs}_{i''}(t'')$. 
    Notice $\OO^\text{obs}_{i''}(t'')\subset\cup_{i\in\I}\Oobs(t'')$, then $\E(t'',z_0,p)\cap \big(\cup_{i\in\I}\Oobs(t'')\big)$.
    Therefore $t''\in\A_1$, which implies $\A_2\subseteq\A_1$.
\end{proof}

\begin{lem}
\label{lem: boole's ineq}
    Suppose the ego vehicle starts with initial condition $z_0\in\Z_0$ and control parameter $p\in\PP$, then
    \begin{equation}
        \begin{split}
            \prob\big(\{t\in[0,\tf]\mid \E(t,z_0,p)\cup\big(\cup_{i\in\I}\Oobs(t)\big)  \} \neq\emptyset  \big)\leq\\
            \leq\sum_{i\in\I}\sum_{j\in\J}\prob(\{t\in T_j\mid \E(t,z_0,p)\cap\Oobs(t) \}\neq\emptyset).
        \end{split}
    \end{equation}
\end{lem}
\begin{proof}
    For notional simplicity, let $\A_3:= \{t\in[0,\tf]\mid \E(t,z_0,p)\cup\big(\cup_{i\in\I}\Oobs(t)\big)  \}$ and $\A_4:=\cup_{j\in\J}\cup_{i\in\I}\{t\in T_j\mid \E(t,z_0,p)\cap\Oobs(t) \}$, then
    \begin{equation}
        \A_3\subseteq \cup_{j\in\J}\{t\in T_j\mid \E(t,z_0,p)\cup\big(\cup_{i\in\I}\Oobs(t)\big)  \} = \A_4
    \end{equation}
    in which the first inclusion follows from the fact that $[0,\tf]\subseteq\cup_{j\in\J} T_j$, and the second equality follows from Lemma \ref{lem: bring cup_i out}.
    Because $\A_3\neq\emptyset$ sufficiently implies $\A_4\neq\emptyset$, then by monotonicity of probability measure
    \begin{equation}
        \prob(\A_3\neq\emptyset) \leq \prob(\A_4\neq\emptyset).
    \end{equation}
    Therefore the claim follows using Boole's inequality \cite{nemirovski2007}.
\end{proof}

Now we state the proof Theorem \ref{thm: risk condition}.
\begin{proof}
    It suffices to show that 
    \begin{equation}
    \label{eq: prob to pdf integrtion}
        \begin{split}
            \prob\big(\{t\in[0,\tf]\mid \E(t,z_0,p)\cup\big(\cup_{i\in\I}\Oobs(t)\big)  \} \neq\emptyset  \big)\leq\\
            \leq \sum_{i\in\I}\sum_{j\in\J}\int_{\xi_i(z_0,p)\oplus\zonocg{0}{\Gobs}}\pdf(w)~dw.
        \end{split}
    \end{equation}
    
    For any $(i,j)\in\I\times\J$, because $\cup_{t\in T_j}\E(t,z_0,p) \subseteq \xi_j(z_0,p) $ by Assumption \ref{ass: offline reachability}, then $\{t\in T_j\mid \E(t,z_0,p) \cup \Oobs(t)\}\neq\emptyset$ implies that 
    \begin{equation}
    \label{eq: relax thru xi}
        \{t\in T_j\mid \xi_j(z_0,p) \cup \Oobs(t)\}\neq\emptyset.
    \end{equation}
    Additionally, by definition of $\wobs$ and Assumption \ref{ass: swept_volume assumption}, \eqref{eq: relax thru xi} implies that $\xi_i(z_0,p)\cap\zonocg{\wobs}{\Gobs}\neq\emptyset$.
    Therefore by monotonicity of probability measure,
    \begin{equation}
    \label{eq: prob for dropping t}
        \begin{split}
            \prob(\{t\in T_j&\mid \E(t,z_0,p)\cap\Oobs(t) \}\neq\emptyset) \leq \\
            &\leq\prob(\xi_i(z_0,p)\cap\zonocg{\wobs}{\Gobs}\neq\emptyset).
        \end{split}
    \end{equation}
    Notice 
    \begin{equation}
    \label{eq: pdf integration to prob}
        \begin{split}
            & \int_{\xi_i(z_0,p)\oplus\zonocg{0}{\Gobs}}\pdf(w)~dw \\
         =  & \prob(\wobs\in\xi_i(z_0,p)\oplus\zonocg{0}{\Gobs})\\
         =  & \prob(\xi_i(z_0,p)\cap\zonocg{\wobs}{\Gobs}\neq\emptyset)
        \end{split}
    \end{equation}
    in which the first equality follows from the definition of probability density function, and the second equality follows from \cite[Lem. 5.1]{guibas2003zonotopes}.
    Therefore \eqref{eq: prob to pdf integrtion} follows from Lemma \ref{lem: boole's ineq}, \eqref{eq: prob for dropping t} and \eqref{eq: pdf integration to prob}.

\end{proof}

%%%%%%%%%%%%%%%%%%%%%%%%%%%%%%%%%%%%%%%%%%%%%%%%%%%%%%%%%%%%%%%%%%%%%%%%%%%%%%%%%%%
\section{Proof of Theorem \ref{thm: risk condition} - OLD}
\label{app: proof of thm risk cond - old}
\jinsun{This is for the OLD version of collision risk with $\wobs$ giving the $i$-th obstacle's location at the middle time of $T_j$}
\begin{proof}
    Notice that 
     \begin{align}
        &\cup_{t\in[0,\tf]}\Big(\E\big(t,z_0,p\big) \cap \big(\cup_{i\in\I}\Oest_i(t)\big) \Big) \nonumber\\
        =& \cup_{j\in\J}\cup_{t\in T_j}\Big(\E\big(t,z_0,p\big) \cap \big(\cup_{i\in\I}\Oest_i(t)\big) \Big)\\
        =& \cup_{j\in\J}\cup_{i\in\I}\cup_{t\in T_j}\Big(\E\big(t,z_0,p\big) \cap \Oest_i(t) \Big)\\
        \subseteq & \cup_{j\in\J}\cup_{i\in\I}\big(\cup_{t\in T_j}\E(t,z_0,p)\big)\cap\big(\cup_{t\in T_j}\Oest_i(t)\big). \label{eq: inclusion} % https://math.stackexchange.com/questions/199349/does-a-cup-b-capc-cup-d-a-cap-c-cupb-cap-d
    \end{align}
    For simplicity let $\texttt E_1$ denote the event of $\cup_{t\in[0,\tf]}\Big(\E\big(t,z_0,p\big) \cap \big(\cup_{i\in\I}\Oest_i(t)\big) \Big)\neq\emptyset$, and let $\texttt E_2$ denote the event of $\cup_{j\in\J}\cup_{i\in\I}\big(\cup_{t\in T_j}\E(t,z_0,p)\big)\cap\big(\cup_{t\in T_j}\Oest_i(t)\big)\neq\emptyset$.
    Because $\texttt E_1$ being true ensures $\texttt E_2$ being true based on \eqref{eq: inclusion}, then by monotonicity of probability measure,
    \begin{equation}
        \prob(\texttt E_1)\leq\prob(\texttt E_2).
    \end{equation}
    Therefore $\prob(\texttt E_2)\leq\epsilon$ implies $\prob(\texttt E_1)\leq\epsilon$.
    Notice by Boole's inequality \cite{nemirovski2007}, 
    \begin{equation}
    \label{ineq: prob <= eps}
    \begin{split}
        &\sum_{i\in\I}\sum_{j\in\J}\prob\Big(\big(\cup_{t\in T_j}\E(t,z_0,p)\big)\cap\\
        &\hspace{3.3cm}\cap\big(\cup_{t\in T_j}\Oest_i(t)\big) \neq\emptyset\Big)\leq\epsilon.
    \end{split}
    \end{equation}
    is a sufficient condition of $\prob(\texttt E_2)\leq\epsilon$, thus it suffices to show that \eqref{ineq: pdf relaxation} sufficiently implies \eqref{ineq: prob <= eps}.

    % By Theorem \ref{thm:footprint}, $\cup_{t\in T_j}\E\big(t,z_0,p\big)\subset\xi(\RR_j,z_0,p)$ for arbitrary $j\in\J$, thus
    By Assumption \ref{ass: offline reachability}, $\cup_{t\in T_j}\E\big(t,z_0,p\big)\subset\xi_j(z_0,p)$ for arbitrary $j\in\J$, thus
    \begin{equation}
    \label{ineq: int_Eps <= int_xi}
        \begin{split} &\sum_{i\in\I}\sum_{j\in\J}\int_{\cup_{t\in T_j}\E\big(t,z_0,p\big)\oplus\zonocg{0}{\Gobs}} \pdf(w) ~dw \leq \\
        &\leq\sum_{i\in\I}\sum_{j\in\J}\int_{\xi_j(z_0,p)\oplus\zonocg{0}{\Gobs}} \pdf(w) ~dw \leq\epsilon.
        \end{split}
    \end{equation}
    Notice by Assumption \ref{ass: obs pdf}, $\pdf(\w)$ describes the probability density of $\w$ during $T_j$, thus 
    \begin{equation}
    \begin{split}
        &\int_{\cup_{t\in T_j}\E(t,z_0,p)\oplus\zonocg{0}{\Gobs}} \pdf(w) ~dw =\\
        &\hspace{0.5cm}=\prob\big( \w\in\cup_{t\in T_j}\E(t,z_0,p)\oplus\zonocg{0}{\Gobs}\big).
    \end{split}
    \end{equation}
    % Recall that by \cite[Lem. 5.1]{guibas2003zonotopes} $\big(\cup_{t\in T_j}\E(z(t),z_0,p)\big)\cap\zonocg{w}{\Gobs} \neq\emptyset$ if and only if $w\in\cup_{t\in T_j}\E(z(t),z_0,p)\oplus\zonocg{0}{\Gobs}$, thus
    Then as a result of \cite[Lem. 5.1]{guibas2003zonotopes},
    \begin{equation}
    \label{eq: int to prob}
    \begin{split}
        &\int_{\cup_{t\in T_j}\E(t,z_0,p)\oplus\zonocg{0}{\Gobs}} \pdf(w) ~dw =\\
        &= \prob\Big(\big(\cup_{t\in T_j}\E(t,z_0,p)\big)\cap\zonocg{\w}{\Gobs} \neq\emptyset\Big).
    \end{split}
    \end{equation}

    % Notice $\cup_{t\in T_j} \Oest_i(t)\subset \zonocg{\w}{\Gobs}$ by Assumption \ref{ass: swept_volume assumption}.
    For simplicity denote $\mathtt E_3$ the event that $\big(\cup_{t\in T_j}\E(t,z_0,p)\big)\cap\zonocg{\w}{\Gobs} \neq\emptyset$, and denote $\mathtt E_4$ the event that $\big(\cup_{t\in T_j}\E(t,z_0,p)\big)\cap\big(\cup_{t\in T_j}\Oest_i(t)\big) \neq\emptyset$.
    Because $\mathtt E_4$ being true sufficiently ensures $\mathtt E_3$ being true due to $\cup_{t\in T_j} \Oest_i(t)\subset \zonocg{\w}{\Gobs}$ by Assumption \ref{ass: swept_volume assumption}, 
    % , and denote $\mathtt E_5$ the event that $\big(\cup_{t\in T_j}\E(z(t),z_0,p)\big)\cap\big(\zonocg{w_i}{\Gobs}\setminus\big(\cup_{t\in T_j}\Oest_i(t)\big) \big)\neq\emptyset$ where `$\setminus$' is the operation of set subtraction.
    % Notice $\mathtt E_3 = \mathtt E_4\cup \mathtt E_5$, 
    then by monotonicity of probability measure 
    \begin{equation}
    \label{ineq: prob mono}
        \prob(\mathtt E_4)\leq\prob(\mathtt E_3).
    \end{equation}
    % see https://math.stackexchange.com/questions/2619834/how-to-show-that-pa-%E2%88%A9-b-%E2%89%A4-pa-%E2%89%A4-pa-%E2%88%AA-b
    Therefore \eqref{ineq: prob <= eps} holds based on \eqref{ineq: int_Eps <= int_xi}, \eqref{eq: int to prob} and \eqref{ineq: prob mono}. 
    % \begin{equation}
    % \label{ineq: prob over Irisk}
    % \begin{split}
    %     &\sum_{i\in\I}\sum_{j\in\J}\prob\Big(\big(\cup_{t\in T_j}\E(t,z_0,p)\big)\cap\\
    %     &\hspace{2.5cm}\cap\big(\cup_{t\in T_j}\Oest_i(t)\big) \neq\emptyset\Big)\leq\epsilon.
    % \end{split}
    % \end{equation}
    % Notice that the set intersection constraints in \opt{} ensure 
    % \begin{equation}
    % \label{eq: prob over Inorisk}
    %     \prob\Big(\big(\cup_{t\in T_j}\E(t,z_0,p)\big)\cap\big(\cup_{t\in T_j}\Oest_i(t)\big) \neq\emptyset\Big) \leq\eta
    % \end{equation}
    % for all $i\in\Inorisk$ by Assumption \ref{ass: uncertainty_overapp}, thus \eqref{ineq: prob <= eps} follows by iteratively adding \eqref{eq: prob over Inorisk} to \eqref{ineq: prob over Irisk} for all $i\in\Inorisk$.

    % \begin{equation}
    %     \begin{split}
    %         \cup_{t\in[0,\tf]}\Big(\E\big(z(t),z_0,p\big) \cap \big(\cup_{i\in\I}\Oest_i(t)\big) \Big) = \\
    %         = \cup_{j\in\J}\cup_{i\in\I}
    %     \end{split}
    % \end{equation}
    
    % Recall by assumption $\int_{\xi(\RR_j,z_0,p)\oplus\zonocg{0}{\Gobs}} f(w) ~dw \leq\epsp$, for all $j\in\J$ and $i\in\I$.
    % Then by the fact that $\cup_{j\in\J} T_j=[0,\tf]$ we have
    % \begin{equation}
    %     \prob\Big(\E\big(z(t),z_0,p\big)  \cap\OO_i(t) \neq\emptyset\Big)\leq\epsp, ~\forall i\in\I, \forall t\in [0,\tf].
    % \end{equation}
    % Therefore by Definition \ref{defn:notatfault-risk} the ego vehicle is not-at-fault with confidence level at least $1-\epsp$ during $[0,t_f]$.
\end{proof}

% \section{Proof of Theorem \ref{thm: risk condition updated}}
% \label{app: proof of thm risk cond updated}
% Through the same reasoning as in the proof of Theorem \ref{thm: risk condition}, it suffices to show that 
% \begin{equation}
% \label{ineq: prob <= eps updated}
% \begin{split}
%     &\sum_{i\in\I}\sum_{j\in\J}\prob\Big(\big(\cup_{t\in T_j}\E(t,z_0,p^*)\big)\cap\\
%     &\hspace{0.3cm}\cap\big(\cup_{t\in T_j}\OO_i(t)\big) \neq\emptyset\Big)\leq\epsp + |\Inorisk||\J|\eta.
% \end{split}
% \end{equation}
% In addition, as an analog to \eqref{ineq: int_Eps <= int_xi} we have
% \begin{equation}
% \label{ineq: int_Eps <= int_xi updated}
%     \begin{split} &\sum_{i\in\Irisk}\sum_{j\in\J}\int_{\cup_{t\in T_j}\E\big(t,z_0,p\big)\oplus\zonocg{0}{\Gobs}} \pdf(w) ~dw \leq \\
%     &\leq\sum_{i\in\Irisk}\sum_{j\in\J}\int_{\xi_j(z_0,p)\oplus\zonocg{0}{\Gobs}} \pdf(w) ~dw \leq\epsp.
%     \end{split}
% \end{equation}
% Notice that the set intersection constraints in \optCV{} ensure 
% \begin{equation}
% \label{eq: prob over Inorisk}
%     \prob\Big(\big(\cup_{t\in T_j}\E(t,z_0,p^*)\big)\cap\big(\cup_{t\in T_j}\Oest_i(t)\big) \neq\emptyset\Big) \leq\eta
% \end{equation}
% for all $i\in\Inorisk$ by Assumption \ref{ass: uncertainty_overapp}.
% Then based on \eqref{eq: int to prob}, \eqref{ineq: prob mono} and the fact that $\I = \Inorisk\cup\Irisk$, \eqref{ineq: prob <= eps updated} follows by iteratively adding \eqref{eq: prob over Inorisk} to \eqref{ineq: int_Eps <= int_xi updated} for all $i\in\Inorisk$ and for all $j\in\J$.
